# Supplementary material for: Text-to-Image Generation for Abstract Concepts
Source: arXiv:2309.14623 source file (2023-09-27)
Supplement: Supplementary file 1 [file 6_appendix.tex]

\appendix
\begin{figure*}[!h]
    \centering
    \includegraphics[width=\textwidth]{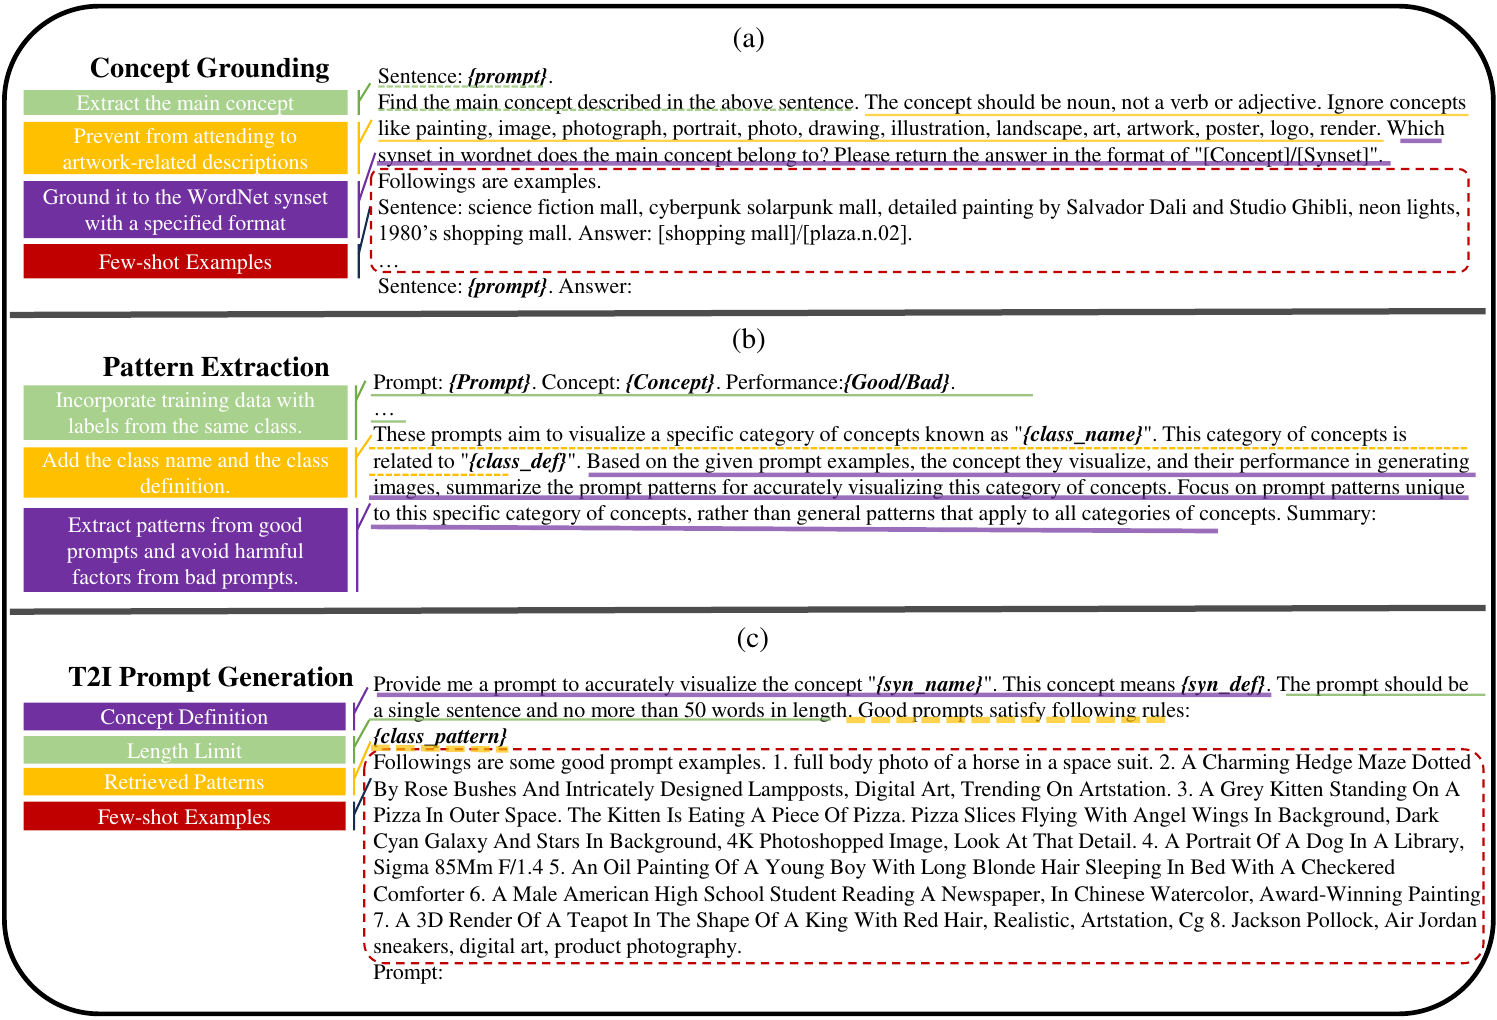}
    % \vspace{-20pt}
    \caption{Detailed LLM prompts. (a) The prompt for the \textit{\underline{Concept Grounding}} step in the \textbf{Form Extraction} stage. (b) The prompt for the \textit{\underline{Pattern Extraction}} step in the \textbf{Form Extraction} stage. (c) The prompt for the \textbf{Prompt Generation} stage.}
    \label{fig:prompt_template}
    % \vspace{-10pt}
\end{figure*}

\begin{figure*}[!h]
    \centering
    \includegraphics[width=\textwidth]{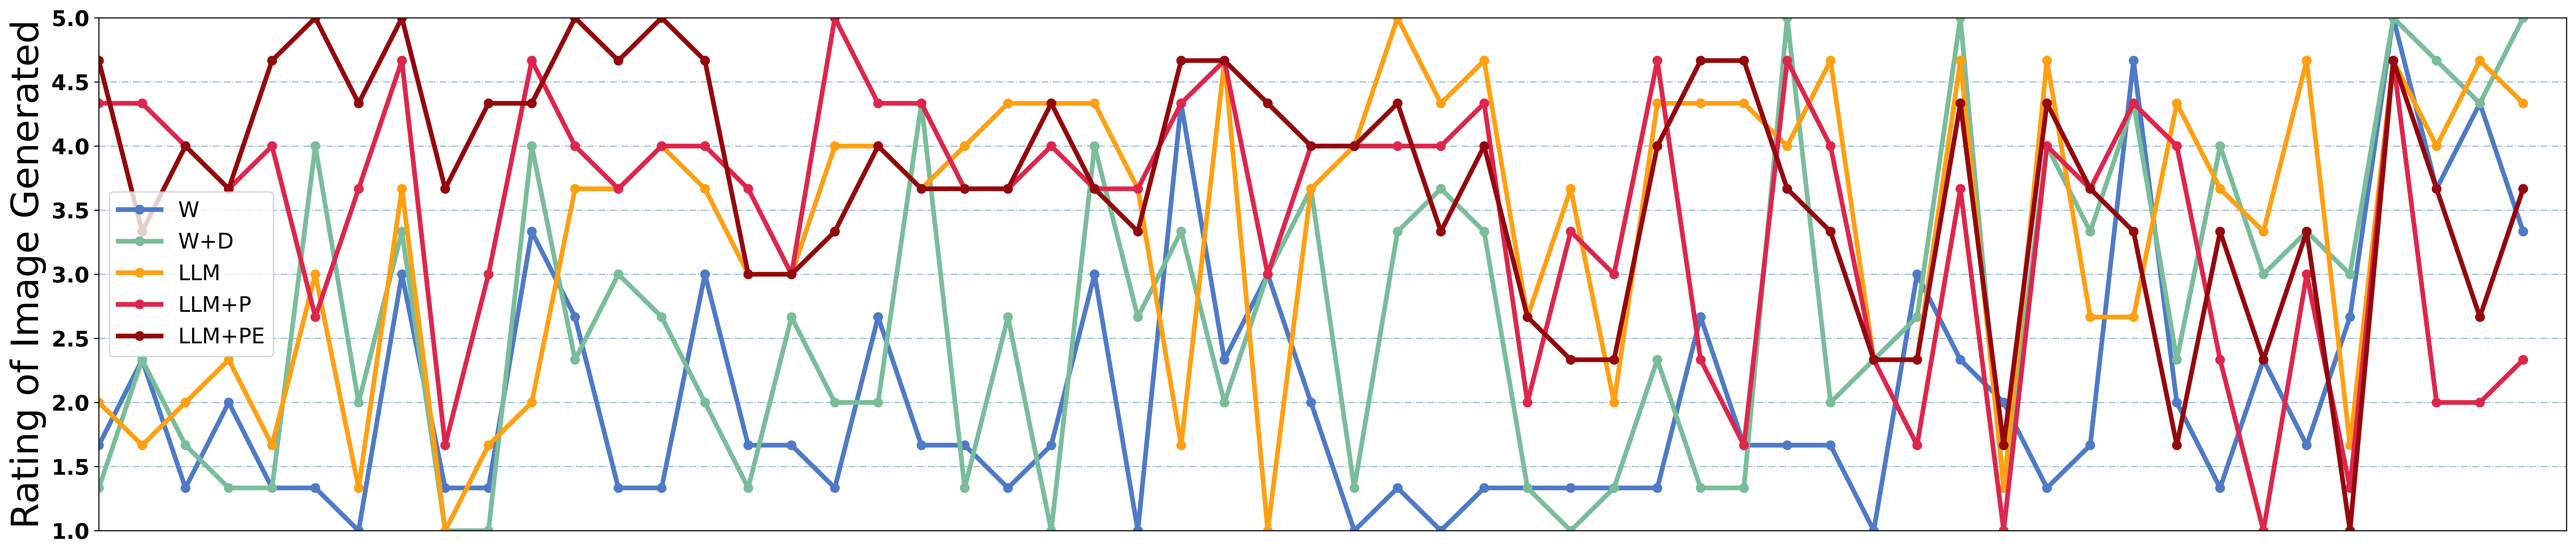}
    % \vspace{-10pt}
    \caption{Details for human evaluation on the small-scale dataset (57 concepts in total). The lines represent the average ratings from three respondents for each concept-images query. }
    \label{fig:human_eval}
    % \vspace{-5pt}
\end{figure*}
\section{Prompts in TIAC}
LLMs are used in multiple stages during the process of creating images for abstract concepts in our framework, which involves multiple LLM prompts. In Figure~\ref{fig:prompt_template}, we provide the detailed prompts in TIAC for reproducing our results. The \textit{prompt} in Figure~\ref{fig:prompt_template} (a)-(b) refers to human-submitted prompts in the SAC dataset. And the \textit{prompt} in Figure~\ref{fig:prompt_template} (c) refers to the refined T2I prompt generated by our framework.

\section{Experiment Details}
\subsection{Human Evaluation on Small-Scale Datasets}
We conduct a survey-based human evaluation on the small-scale dataset, consisting of 57 questionnaire sections corresponding to 57 abstract concepts. The name of the concept and its definition from WordNet is presented at the beginning of each section. There are five questions in one section, each in the format of ``Image-Ranking choice". To alleviate the randomness in Stable Diffusion, we generate three images for one prompt and group them in a row, and there are five rows of images for one abstract concept representing the five types of prompts mentioned above. Participants were asked to rate the generated images for each row on a scale of 1 to 5 based on their sense, with 5 being the best and 1 being the worst. The link to our survey is \url{https://forms.gle/ke7cDY1kfKwJmcmz5}.
By the way, we also paid each participant the fee (based on the local average hourly wage) for completing the survey.

The detailed human assessment results for each abstract concept are illustrated in Figure \ref{fig:human_eval}.
Notably, the results indicate that LLM+PE and LLM+P (lines colored red) usually score higher, revealing a preference for the images generated by our framework in the majority of cases, as perceived by humans.

\subsection{Results on Large-Scale Datasets}
We also evaluate performance on the large-scale dataset from the granularity of the subclass. Here, subclass nodes are the direct children of the seven classes we mention in Section \textbf{Concept Class Determination}. For each subclass, the number of corresponding prompts in SAC is over 10, and the number of its children in WordNet is over 100. The results of using concept score as the evaluation metric are organized in Table~\ref{tab:large_eval}. It shows that in most cases (33/34 subclasses), the concept score on images generated by prompts from our framework (LLM+P and LLM+PE) is higher than other baselines, demonstrating the effectiveness in both the design for the text-to-image generation for abstract concepts task and the evaluation metric in measuring human preference on generated images.

%\begin{figure}[t]
%    \centering
    %\includegraphics[width=0.5\textwidth]{charts/appendix_concept_grounding.pdf}
%    \vspace{-20pt}
%    \caption{The LLM Prompt for Concept Grounding.}
    %\label{fig:concept_grounding_prompt}
%    \vspace{-10pt}
%\end{figure}

%\begin{figure}[t]
%    \centering
    %\includegraphics[width=0.5\textwidth]{charts/appendix_pattern_extraction.pdf}
%    \vspace{-20pt}
%    \caption{The LLM Prompt for Pattern Extraction.}
    %\label{fig:pattern_extraction_prompt}
%    \vspace{-10pt}
%\end{figure}

%\begin{figure}[t]
%    \centering
%    \includegraphics[width=0.5\textwidth]{charts/appendix_prompt_generation.pdf}
%    \vspace{-20pt}
%    \caption{The LLM Prompt for T2I Prompt Generation.}
%    \label{fig:prompt_generation_prompt}
%    \vspace{-10pt}
%\end{figure}

\begin{table*}[!h]
\centering
\begin{tabular}{c|c|c|c|c|c|c}
\toprule
\textbf{Class}                                                                      & \textbf{Subclass}                                                         & \textbf{W} & \textbf{W+D}       & \textbf{LLM} & \textbf{LLM+P}     & \textbf{LLM+PE}    \\ \midrule
\multirow{5}{*}{\textbf{Attribute}}                                                 & \textbf{Property}                                                         & 0.79±0.01  & 0.82±0.01          & 1.12±0.02    & \textbf{1.41±0.01} & 1.41±0.00             \\ 
& \textbf{Quality}                                                          & 0.69±0.00     & 0.63±0.02          & 0.92±0.02    & \textbf{1.43±0.01} & 1.42±0.00             \\  
& \textbf{Shape}                                                            & 0.98±0.04  & 1.15±0.02          & 1.17±0.01    & \textbf{1.38±0.01} & 1.29±0.01          \\ 
& \textbf{State}                                                            & 0.80±0.01   & 0.87±0.04          & 1.16±0.01    & 1.39±0.01          & \textbf{1.42±0.01} \\ 
& \textbf{Trait}                                                            & 0.65±0.02  & 0.56±0.02          & 0.91±0.02    & \textbf{1.47±0.02} & 1.46±0.00             \\ \midrule
\multirow{5}{*}{\textbf{Cognition}}                                                 & \textbf{Ability}                                                          & 0.86±0.02  & 0.97±0.02          & 1.07±0.01    & 1.35±0.01          & \textbf{1.56±0.02} \\ 
& \textbf{Attitude}                                                         & 0.82±0.03  & 0.76±0.02          & 0.99±0.03    & 1.28±0.01          & \textbf{1.54±0.01} \\ 
& \textbf{Content}                                                          & 0.82±0.02  & 0.96±0.02          & 1.09±0.02    & 1.34±0.01          & \textbf{1.57±0.01} \\ 
& \textbf{Information}                                                      & 0.81±0.01  & 1.05±0.01          & 1.22±0.02    & 1.18±0.02          & \textbf{1.45±0.01} \\  
& \textbf{Process}                                                          & 0.83±0.00     & 0.86±0.03          & 0.98±0.02    & 1.19±0.03          & \textbf{1.50±0.01}  \\ \midrule
\multirow{7}{*}{\textbf{\begin{tabular}[c]{@{}c@{}}Communi-\\ cation\end{tabular}}} & \textbf{\begin{tabular}[c]{@{}c@{}}Auditory \end{tabular}} & 0.86±0.01  & 0.84±0.01          & 1.09±0.02    & 1.31±0.02          & \textbf{1.40±0.02}  \\ 
& \textbf{\begin{tabular}[c]{@{}c@{}}Expressive\end{tabular}}       & 0.81±0.02  & 0.75±0.02          & 0.94±0.03    & 1.28±0.01          & \textbf{1.37±0.01} \\ 
& \textbf{Indication}                                                       & 0.87±0.02  & 0.86±0.02          & 0.95±0.01    & 1.20±0.00              & \textbf{1.28±0.01} \\ 
& \textbf{Language}                                                         & 1.04±0.02  & 1.15±0.03          & 1.19±0.04    & 1.50±0.01           & \textbf{1.58±0.01} \\  
& \textbf{Message}                                                          & 0.74±0.01  & 0.68±0.01          & 0.76±0.01    & 1.22±0.03          & \textbf{1.33±0.01} \\  
& \textbf{Signal}                                                           & 0.96±0.01  & 1.19±0.01          & 1.16±0.01    & 1.27±0.01          & \textbf{1.34±0.01} \\ 
& \textbf{\begin{tabular}[c]{@{}c@{}}Written\end{tabular}}  & 0.78±0.01  & 0.80±0.02           & 1.00±0.01       & 1.23±0.02          & \textbf{1.36±0.02} \\ \midrule
\multirow{4}{*}{\textbf{Event}}                                                     & \textbf{Act}                                                              & 0.83±0.01  & 0.93±0.01          & 1.15±0.02    & 1.39±0.02          & \textbf{1.48±0.00}    \\ 
& \textbf{Group Action}                                                     & 0.84±0.02  & 0.89±0.01          & 1.09±0.01    & 1.36±0.01          & \textbf{1.51±0.01} \\ 
& \textbf{Happening}                                                        & 0.86±0.01  & 0.94±0.03          & 1.07±0.02    & 1.29±0.03          & \textbf{1.44±0.02} \\ 
& \textbf{Social Event}                                                     & 1.16±0.03  & 1.27±0.03          & 1.37±0.01    & 1.47±0.02          & \textbf{1.56±0.01} \\ \midrule
\multirow{5}{*}{\textbf{Group}}                                                     & \textbf{Arrangement}                                                      & 0.82±0.01  & 0.83±0.02          & 0.92±0.02    & 1.29±0.01          & \textbf{1.35±0.01} \\
& \textbf{\begin{tabular}[c]{@{}c@{}}Biological\end{tabular}}       & 1.15±0.02  & \textbf{1.56±0.02} & 1.50±0.01     & 1.54±0.01          & 1.55±0.01          \\ 
& \textbf{Collection}                                                       & 0.98±0.02  & 1.11±0.01          & 1.29±0.03    & 1.40±0.01           & \textbf{1.47±0.01} \\ 
& \textbf{People}                                                           & 0.92±0.01  & 1.09±0.01          & 1.36±0.02    & 1.46±0.02          & \textbf{1.52±0.01} \\  
& \textbf{Social Group}                                                     & 1.10±0.03   & 1.27±0.05          & 1.39±0.01    & 1.53±0.02          & \textbf{1.57±0.01} \\ \midrule
\multirow{4}{*}{\textbf{Measure}}                                                   & \textbf{\begin{tabular}[c]{@{}c@{}}Definite\end{tabular}}      & 0.93±0.00     & 1.05±0.02          & 1.07±0.04    & 1.13±0.01          & \textbf{1.14±0.02} \\ 
& \textbf{\begin{tabular}[c]{@{}c@{}}Fundamental\end{tabular}}   & 0.94±0.03  & 1.10±0.01           & 1.24±0.01    & 1.30±0.02           & \textbf{1.43±0.00}    \\ 
& \textbf{\begin{tabular}[c]{@{}c@{}}Indefinite\end{tabular}}    & 1.06±0.02  & 1.18±0.02          & 1.35±0.03    & \textbf{1.40±0.02}  & 1.37±0.00             \\ 
& \textbf{\begin{tabular}[c]{@{}c@{}}system\end{tabular}}  & 1.00±0.01     & 1.17±0.01          & 1.21±0.02    & 1.23±0.01          & \textbf{1.31±0.01} \\ \midrule
\multirow{4}{*}{\textbf{Relation}}                                                  & \textbf{\begin{tabular}[c]{@{}c@{}}Magnitude\end{tabular}}     & 0.74±0.01  & 0.72±0.00             & 0.91±0.01    & 0.98±0.02          & \textbf{1.25±0.01} \\ 
& \textbf{Part}                                                             & 1.00±0.01     & 1.18±0.02          & 1.27±0.03    & 1.25±0.01          & \textbf{1.37±0.01} \\ 
& \textbf{Position}                                                         & 0.87±0.02  & 0.95±0.02          & 1.20±0.01     & 1.28±0.03          & \textbf{1.45±0.02} \\ 
& \textbf{Possession}                                                       & 0.80±0.02   & 0.85±0.02          & 1.15±0.01    & 1.02±0.03          & \textbf{1.28±0.01} \\ \bottomrule
\end{tabular}
\caption{Evaluation with concept score on the large-scale dataset. \textbf{Bold} value indicates the best performance. Auditory, Expressive, Written, Biological, Definite, Fundamental, Indefinite, System and Magnitude are abbreviations for the concept name of subclass node Auditory Communication, Expressive Style, Written Communication, Biological Group, Definite Quantity, Fundamental Quantity, Indefinite Quantity, System of Measurement and Magnitude Relation, respectively.}
\label{tab:large_eval}
\end{table*}

\section{Case study}
Additionally, we select one abstract concept of each class and display the generated images. We also utilize DALL-E as our image generation model apart from Stable Diffusion 2, which can provide evidence of the generalization ability of our framework across different T2I models.

\begin{figure*}[!h]
    \centering
    \includegraphics[width=0.8\textwidth]{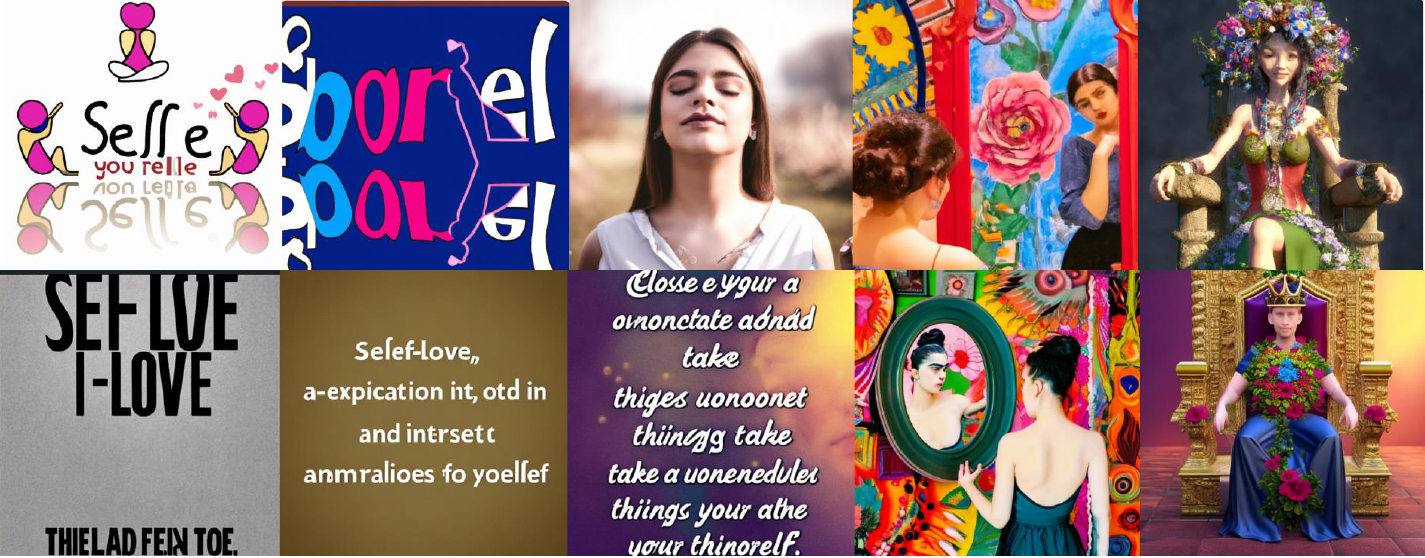}
    \caption{The images generated to convey the concept of ``self-love.n.02'' with five approaches, W, W+D, LLM, LLM+P, LLM+PE, respectively from left to right. The first row is generated by DALL-E, and the second row is generated by Stable Diffusion 2.}
    \label{fig:trait_self-love}
    %\vspace{-10pt}
\end{figure*}

The concept ``self-love.n.02'' belongs to the class ``attribute'' and the subclass ``trait''. The prompts generated are: 
(1) W: self-love; (2) W+D: self-love, an   exceptional interest in and admiration for yourself; (3) LLM: Close your eyes and   take a moment to appreciate all the wonderful things about yourself; (4) LLM+P: A young woman admiring   her reflection in a mirror, surrounded by vibrant colors and artwork inspired   by Frida Kahlo, radiating self-love and confidence; (5) LLM+PE: A 3D Render Of A   Person Sitting On A Throne, Wearing A Crown Of Flowers, With A Radiant Smile,   Artstation, Cg.
Figure~\ref{fig:trait_self-love} shows the images generated.

\begin{figure*}[!h]
    \centering
    \includegraphics[width=0.8\textwidth]{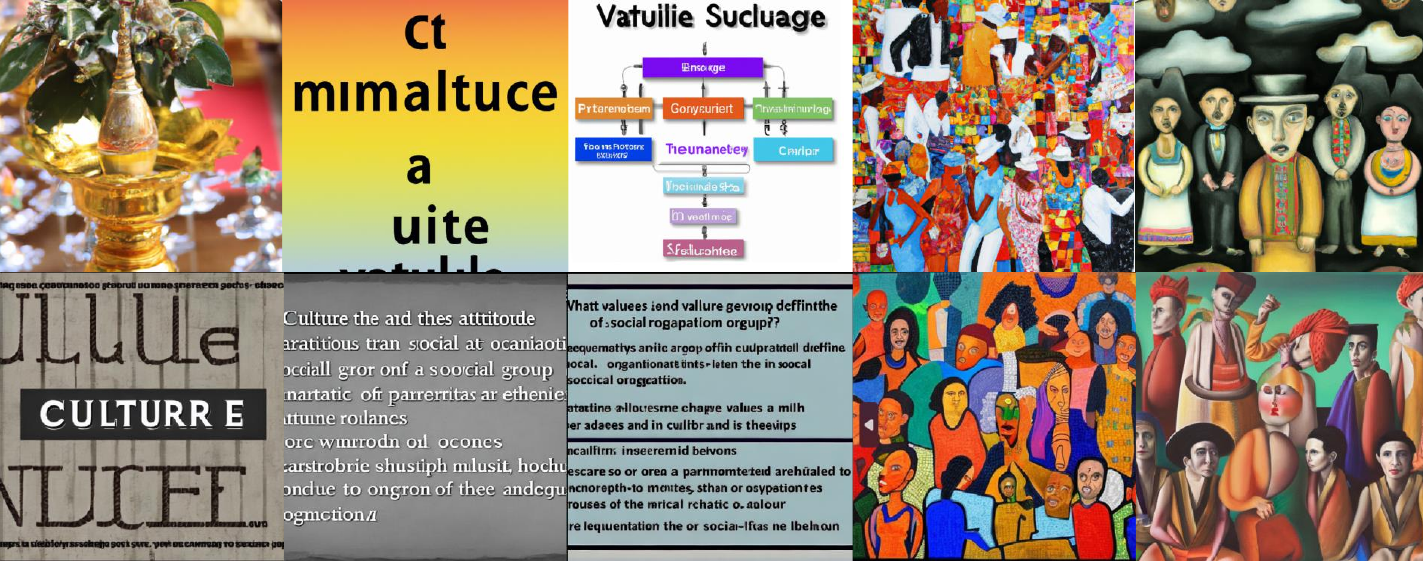}
    \caption{The images generated to convey the concept of ``culture.n.06'' with five approaches, W, W+D, LLM, LLM+P, LLM+PE, respectively from left to right. The first row is generated by DALL-E, and the second row is generated by Stable Diffusion 2.}
    \label{fig:attitude_culture}
    %\vspace{-10pt}
\end{figure*}

The concept ``culture.n.06'' belongs to the class ``communication'' and the subclass ``message''. The prompts generated are: 
(1) W: culture; 
(2) W+D: culture, the attitudes and behavior that are characteristic of a particular social group or   organization; 
(3) LLM: What values and behaviors define the culture of a particular social group or organization? 
(4) LLM+P: A mosaic of diverse   attitudes and behaviors, reflecting the unique culture of a social group,   comes alive in a vibrant painting; 
(5) LLM+PE: A surrealist painting of   a group of people in traditional clothing, each with a unique expression,   representing the culture of a particular social group. 
Figure~\ref{fig:attitude_culture} shows the images generated.

\begin{figure*}[!h]
    \centering
    \includegraphics[width=0.8\textwidth]{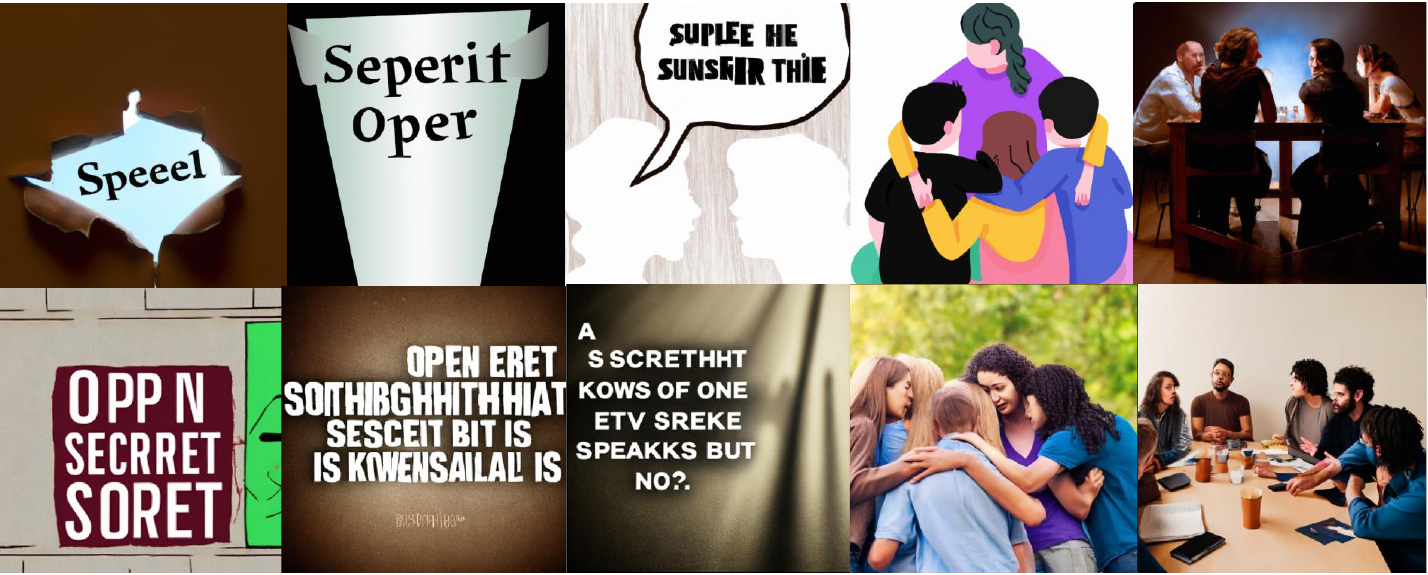}
    \caption{The images generated to convey the concept of ``open\_secrete.n.01'' with five approaches, W, W+D, LLM, LLM+P, LLM+PE, respectively from left to right. The first row is generated by DALL-E, and the second row is generated by Stable Diffusion 2.}
    \label{fig:message_open_secrete}
    %\vspace{-10pt}
\end{figure*}
The concept ``open\_secret.n.01'' belongs to the class ``cognition'' and the subclass ``attitude''. The prompts generated are: (1) W: open\_secret; 
(2) W+D: open\_secret, something that is supposed to be secret but is generally known; 
(3) LLM: A secret that everyone   knows, but no one speaks of; 
(4) LLM+P: A group of people   huddle together, whispering secrets that everyone already knows; (5) LLM+PE: A group of people   gathered around a table, discussing an open secret with hushed tones and   intense expressions. 
Figure~\ref{fig:message_open_secrete} shows the images generated.

\begin{figure*}[!h]
    \centering
    \includegraphics[width=0.8\textwidth]{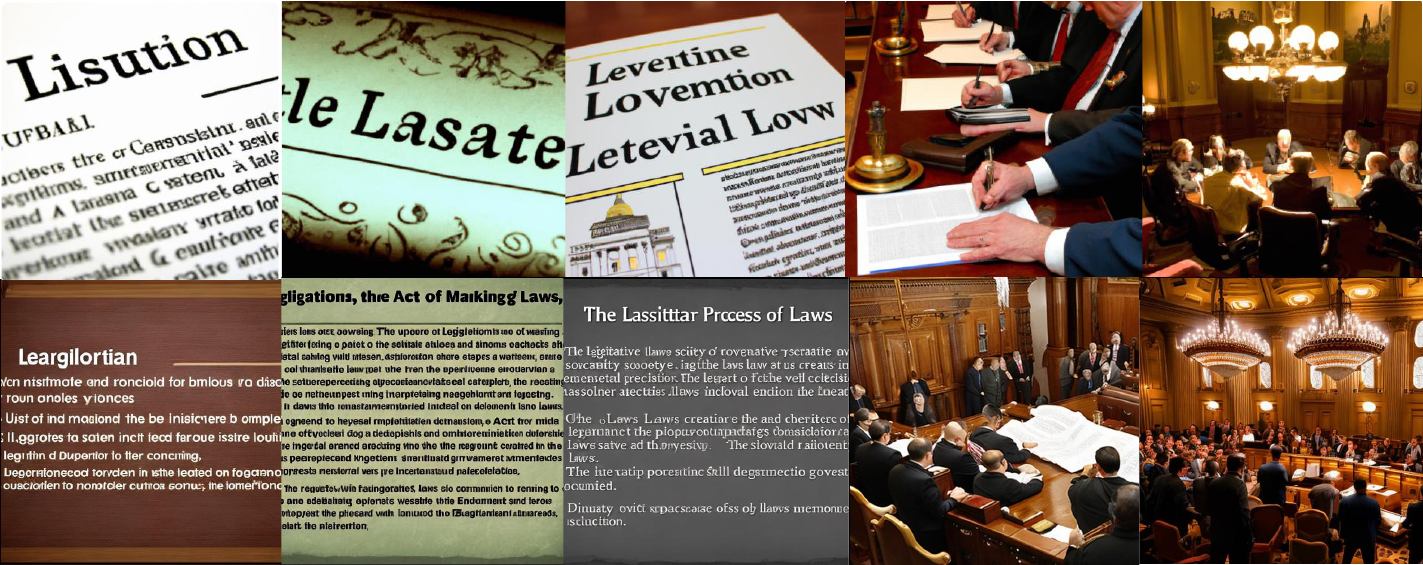}
    \caption{The images generated to convey the concept of ``legislation.n.02'' with five approaches, W, W+D, LLM, LLM+P, LLM+PE, respectively from left to right. The first row is generated by DALL-E, and the second row is generated by Stable Diffusion 2.}
    \label{fig:group_action_legislation}
    %\vspace{-10pt}
\end{figure*}
The concept ``legislation.n.02'' belongs to the class ``event'' and the subclass ``group action''. The prompts generated are:
(1) W: legislation; 
(2) W+D: legislation, the act   of making or enacting laws; 
(3) LLM: The legislative   process of creating laws to govern society; 
(4) LLM+P: In a solemn atmosphere,   legislators gather to enact new laws, their pens scratching against parchment   in a timeless ritual; 
(5) LLM+PE: A group of lawmakers   gathered in a grand hall, debating passionately as they craft new   legislation, illuminated by the warm glow of a chandelier. 
Figure~\ref{fig:group_action_legislation} shows the images generated.

\begin{figure*}[!h]
    \centering
    \includegraphics[width=0.8\textwidth]{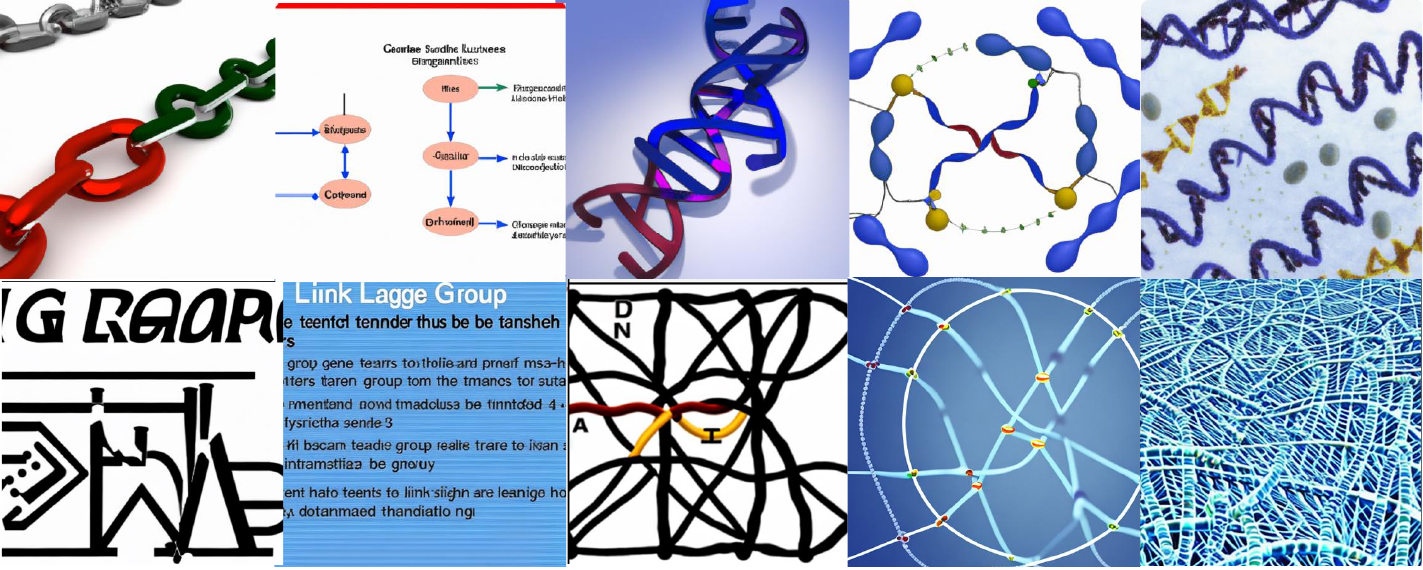}
    \caption{The images generated to convey the concept of ``linkage\_group.n.01'' with five approaches, W, W+D, LLM, LLM+P, LLM+PE, respectively from left to right. The first row is generated by DALL-E, and the second row is generated by Stable Diffusion 2.}
    \label{fig:arragement_linkage_group}
    %\vspace{-10pt}
\end{figure*}
The concept ``linkage\_group.n.01'' belongs to the class ``group'' and the subclass ``arrangement''. The prompts generated are: 
(1) W: linkage\_group; 
(2) W+D: linkage\_group, any   pair of genes that tend to be transmitted together; 
(3) LLM: Two genes connected by   a strong bond, linked together in a group; 
(4) LLM+P: A group of genes   linked together, sharing a common transmission; 
(5) LLM+PE: A group of genes linked   together, forming intricate patterns in a laboratory setting. 
Figure~\ref{fig:arragement_linkage_group} shows the images generated.

\begin{figure*}[!h]
    \centering
    \includegraphics[width=0.8\textwidth]{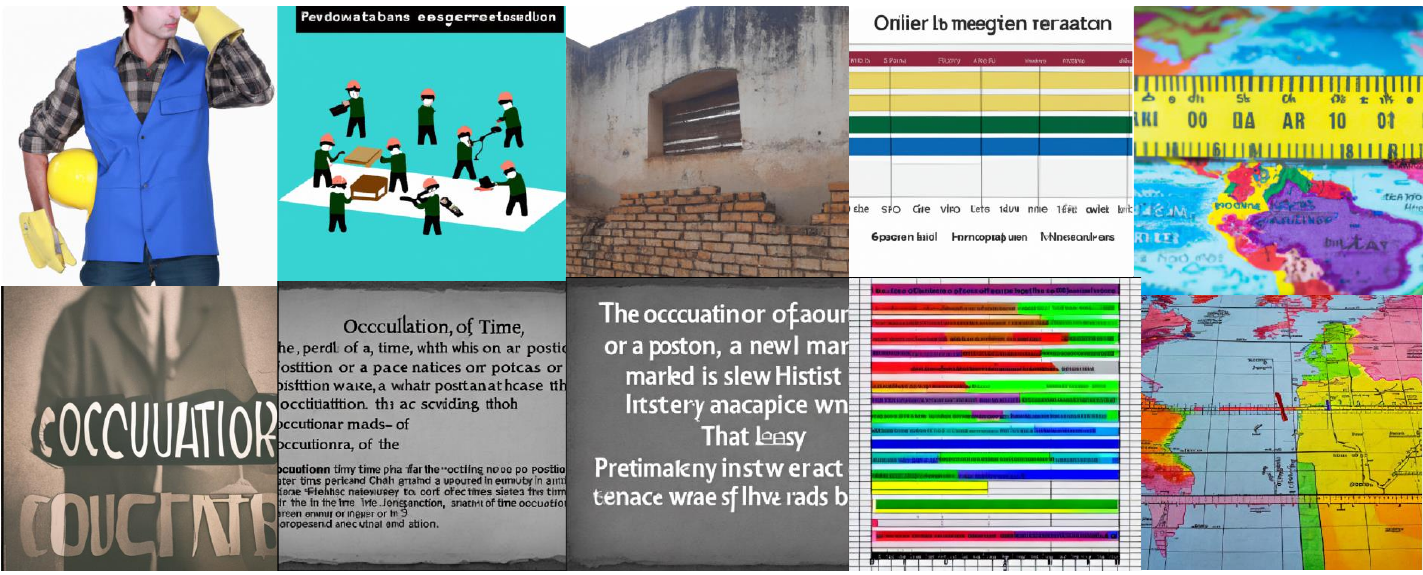}
    \caption{The images generated to convey the concept of ``occupation.n.05'' with five approaches, W, W+D, LLM, LLM+P, LLM+PE, respectively from left to right. The first row is generated by DALL-E, and the second row is generated by Stable Diffusion 2.}
    \label{fig:fundamental_quantity_occupation}
   % \vspace{-10pt}
\end{figure*}
The concept ``occupation.n.05'' belongs to the class ``measure'' and the subclass ``fundamental quantity''. The prompts generated are: 
(1) W: occupation; 
(2) W+D: occupation, the period   of time during which a place or position or nation is occupied; 
(3) LLM: The occupation of a   place or position marked a new era in its history; 
(4) LLM+P: Observe the length of   the occupation of a place or position over time, represented by a ruler with   a timeline of colors; 
(5) LLM+PE: A ruler measuring the   length of a nation's occupation, surrounded by a colorful map of the region.
Figure~\ref{fig:fundamental_quantity_occupation} shows the images generated.

\begin{figure*}[!h]
    \centering
    \includegraphics[width=0.8\textwidth]{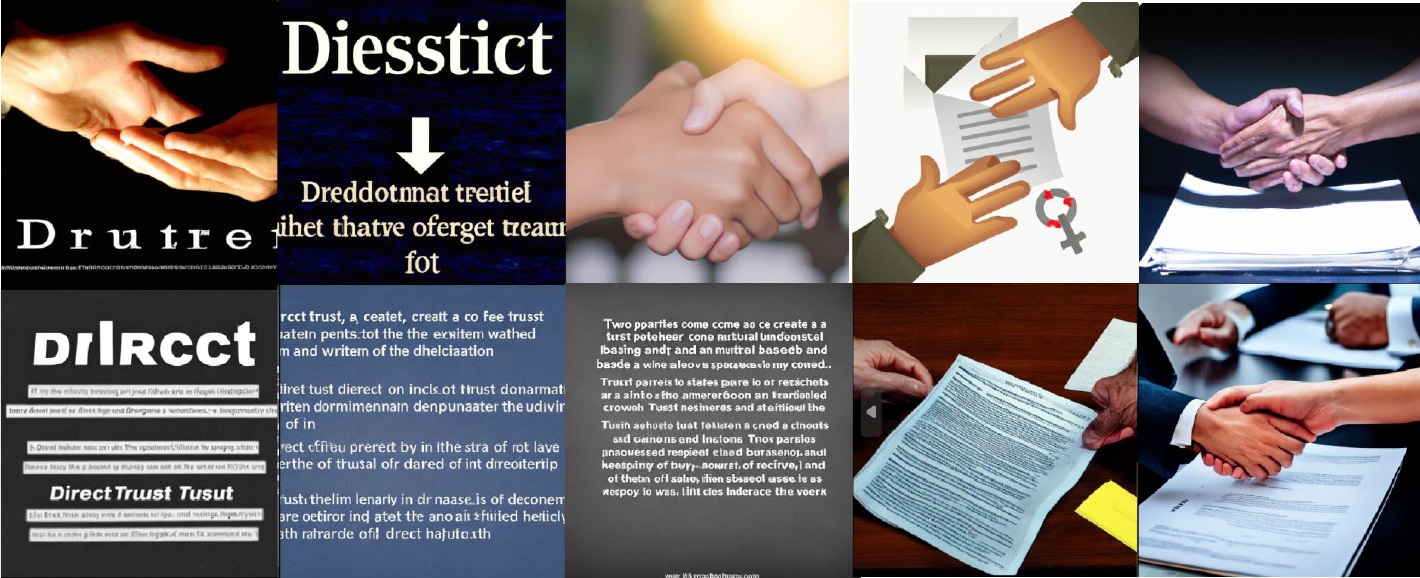}
    \caption{The images generated to convey the concept of ``direct\_trust.n.01'' with five approaches, W, W+D, LLM, LLM+P, LLM+PE, respectively from left to right. The first row is generated by DALL-E, and the second row is generated by Stable Diffusion 2.}
    \label{fig:possession_direct_trust}
   % \vspace{-10pt}
\end{figure*}
The concept ``direct\_trust.n.01'' belongs to the class ``relation'' and the subclass ``possession''. The prompts generated are: 
(1) W: direct\_trust; 
(2) W+D: direct\_trust, a trust   created by the free and deliberate act of the parties involved (usually on   the basis of written documentation); 
(3) LLM: Two parties come   together to create a trust, based on mutual understanding and respect; 
(4) LLM+P: Two parties come   together to create a direct trust, their connection sealed by a mysterious   document; 
(5)LLM+PE: Two hands clasping a   document, symbolizing the direct trust between the parties involved. 
Figure~\ref{fig:possession_direct_trust} shows the images generated.

%The prompt should be a single sentence and no more than 50 words in length. The prompt should contain concrete objects to reveal the concept meaning.  

% \section{Human Subjects}
